# Supplementary material for: On the Uncertain Single-View Depths in Colonoscopies
Source: arXiv:2112.08906 source file (2022-07-20)
Supplement: Supplementary file 1 [file suplementary.tex]

\section*{On the Uncertain Single-View Depths in Colonoscopies -Supplementary Material-}
\pagenumbering{gobble} 
\setcounter{page}{1}
\setcounter{figure}{0}
\begin{figure}%{\textwidth}
  \includegraphics[width=\columnwidth]{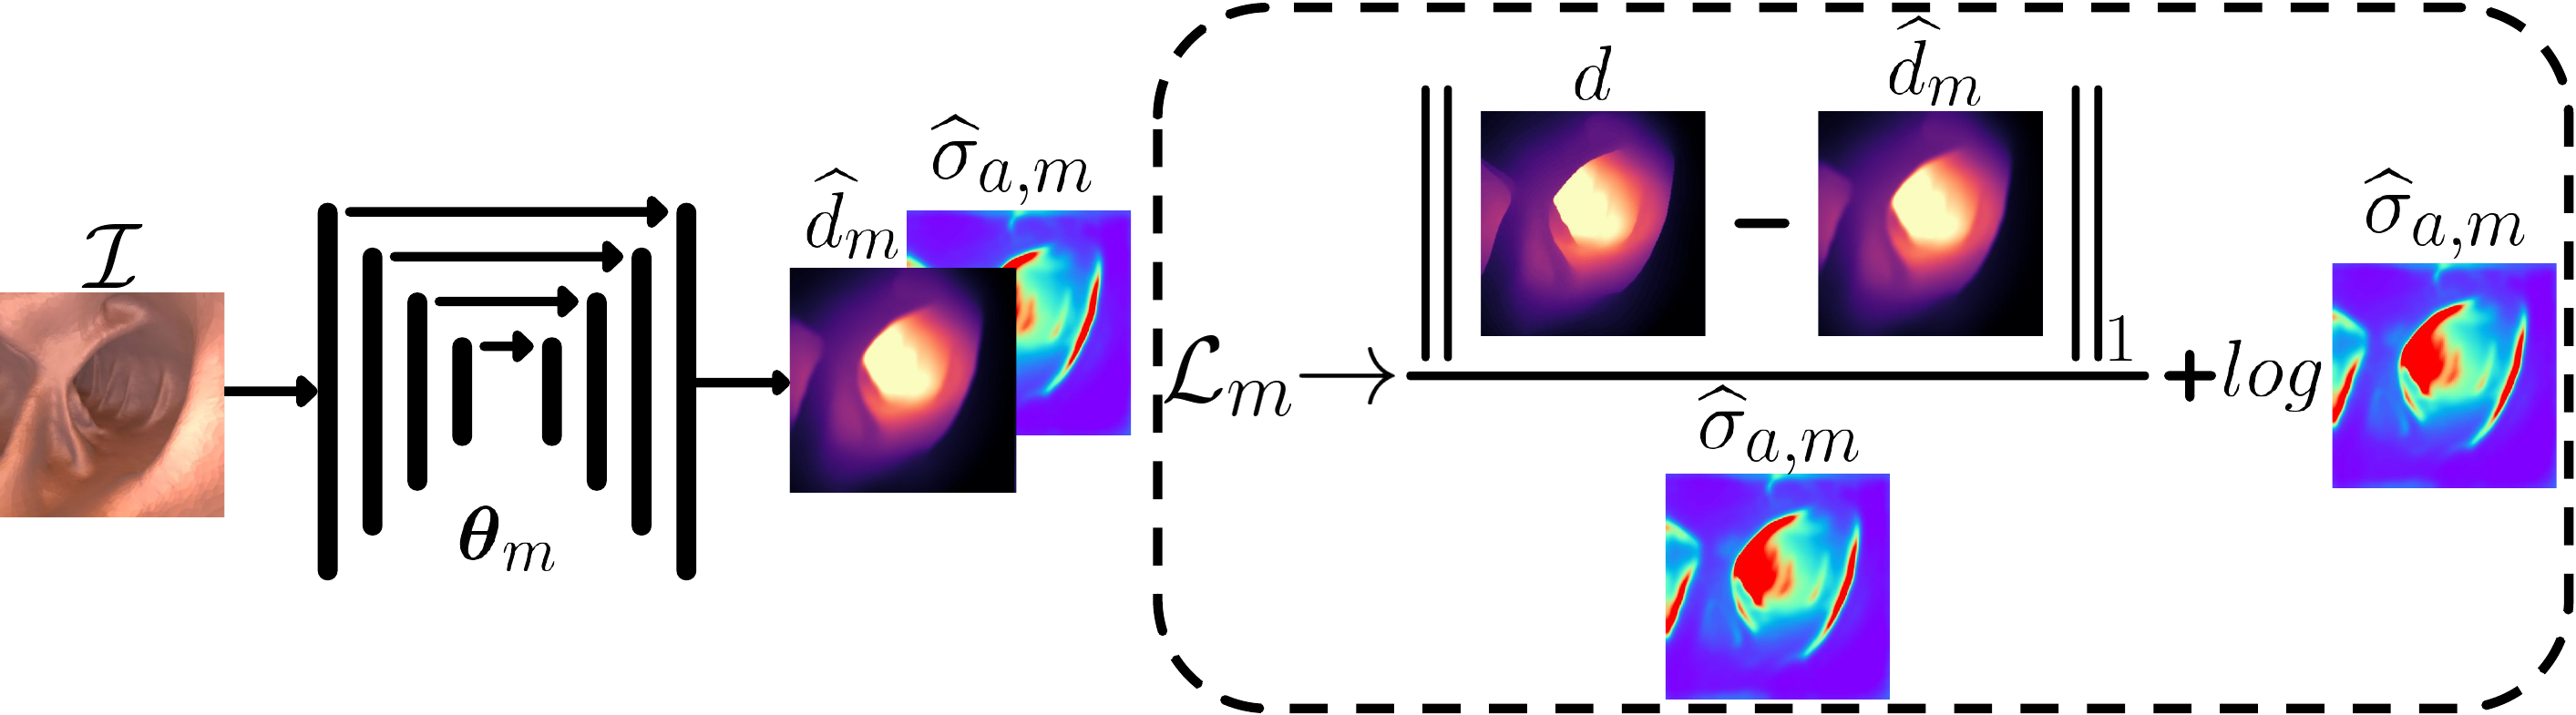}
  \centering
  \caption{Supervised training of a single ensemble \textit{m}. Depth $\widehat{d}_m$ and aleatoric uncertainty $\sigma_{a,m},$ estimation for a target image $\mathcal{I}$. We define graphically the loss for a single ensemble. $\widehat{d}_m$ depth prediction, $d$ depth target  and $\sigma_{a,m}$ the aleatoric uncertainty of the ensemble. }
\label{fig:trainsup}
\end{figure}

\begin{figure}
    \centerline{\includegraphics[width=\columnwidth]{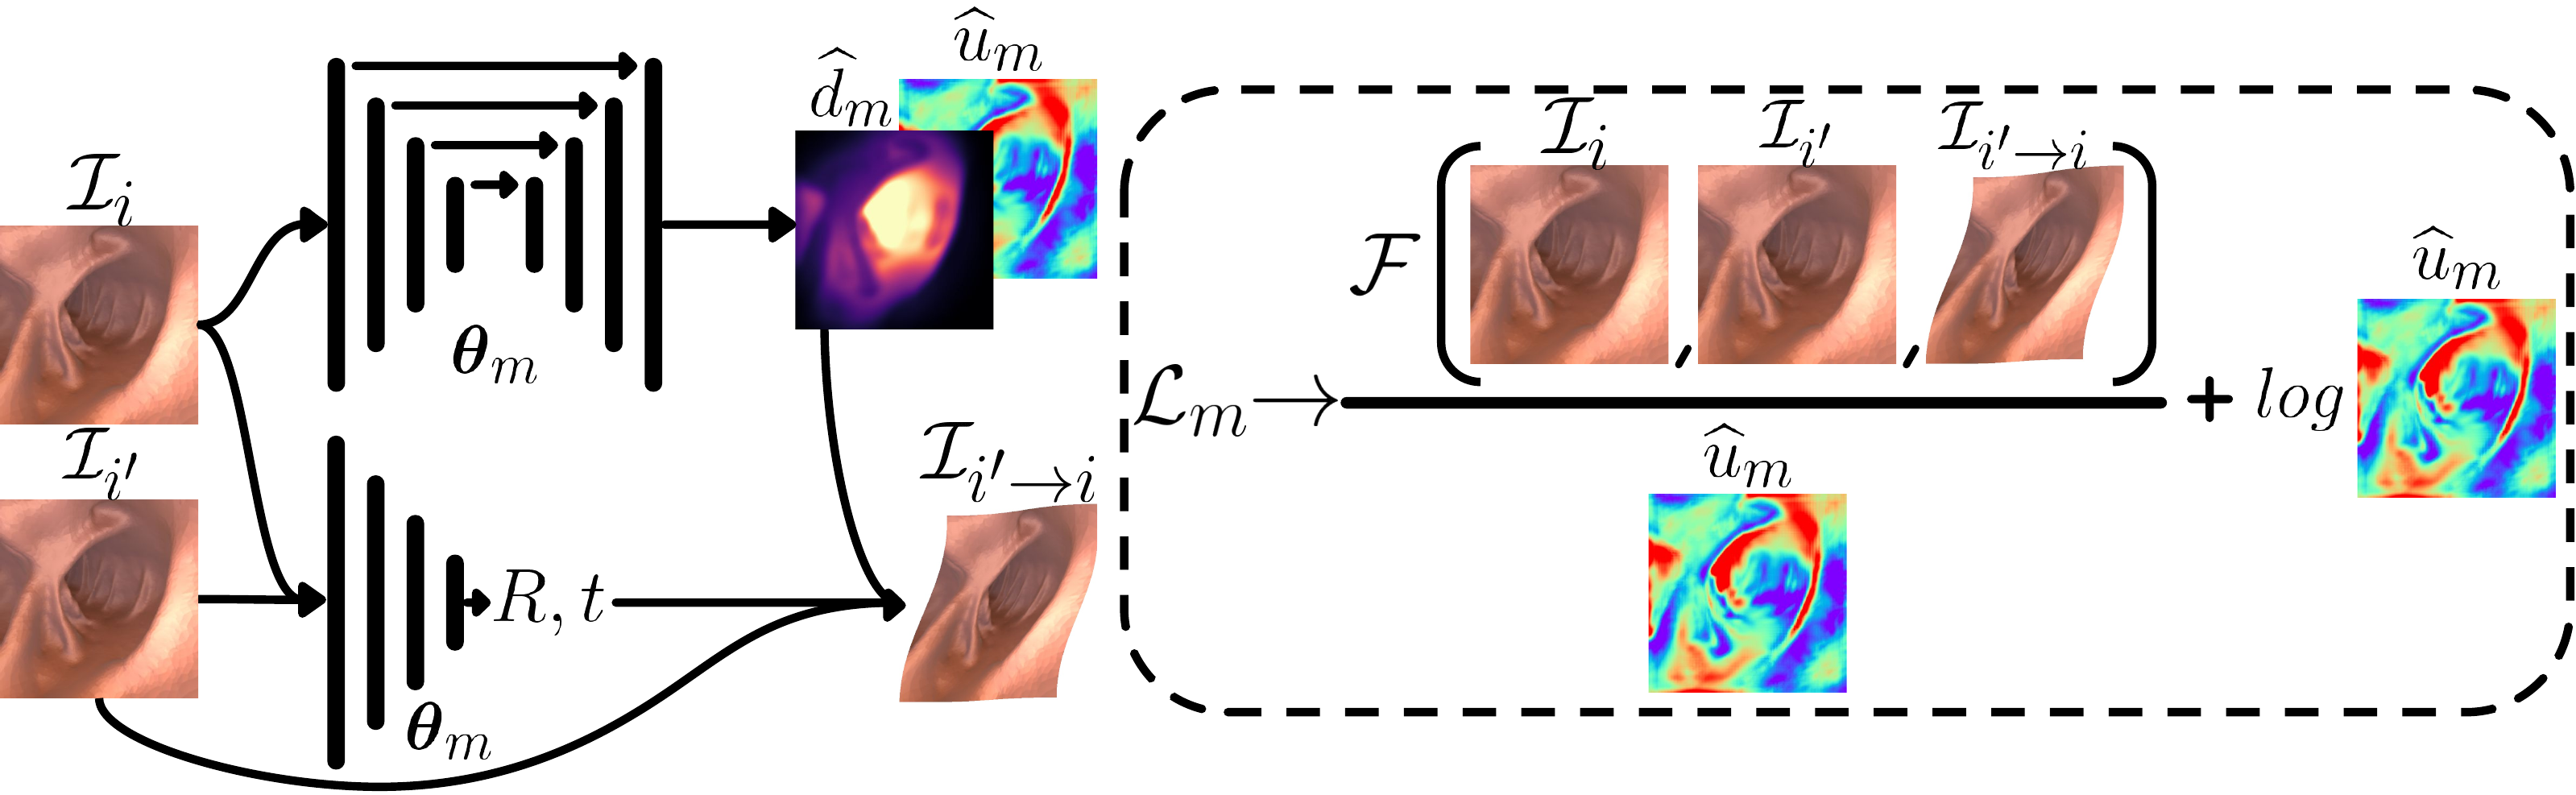}}
    \caption{Self-supervised training of deep ensembles. Each network $m$ in the ensemble learns to predict disparity $\widehat{\underline{d}}$ and observation noise $\widehat{u}_m$, referred to photometric residual, for a target image $\mathcal{I}_i$. A secondary network predicts the relative rotation $\boldsymbol{R}$ and translation $\boldsymbol{t}$ between the target view and several source ones $\mathcal{I}_{i^\prime}$. The predicted depths and camera motion allows to warp the target image to the image plane of the source images $\mathcal{I}_{i^\prime\rightarrow i}$. The loss $\mathcal{L}_m$ depends on a function of the three color images.}
    \label{fig:Approach_Self-Supervised}
\end{figure}
\begin{figure}
    \centerline{\includegraphics[width=\columnwidth]{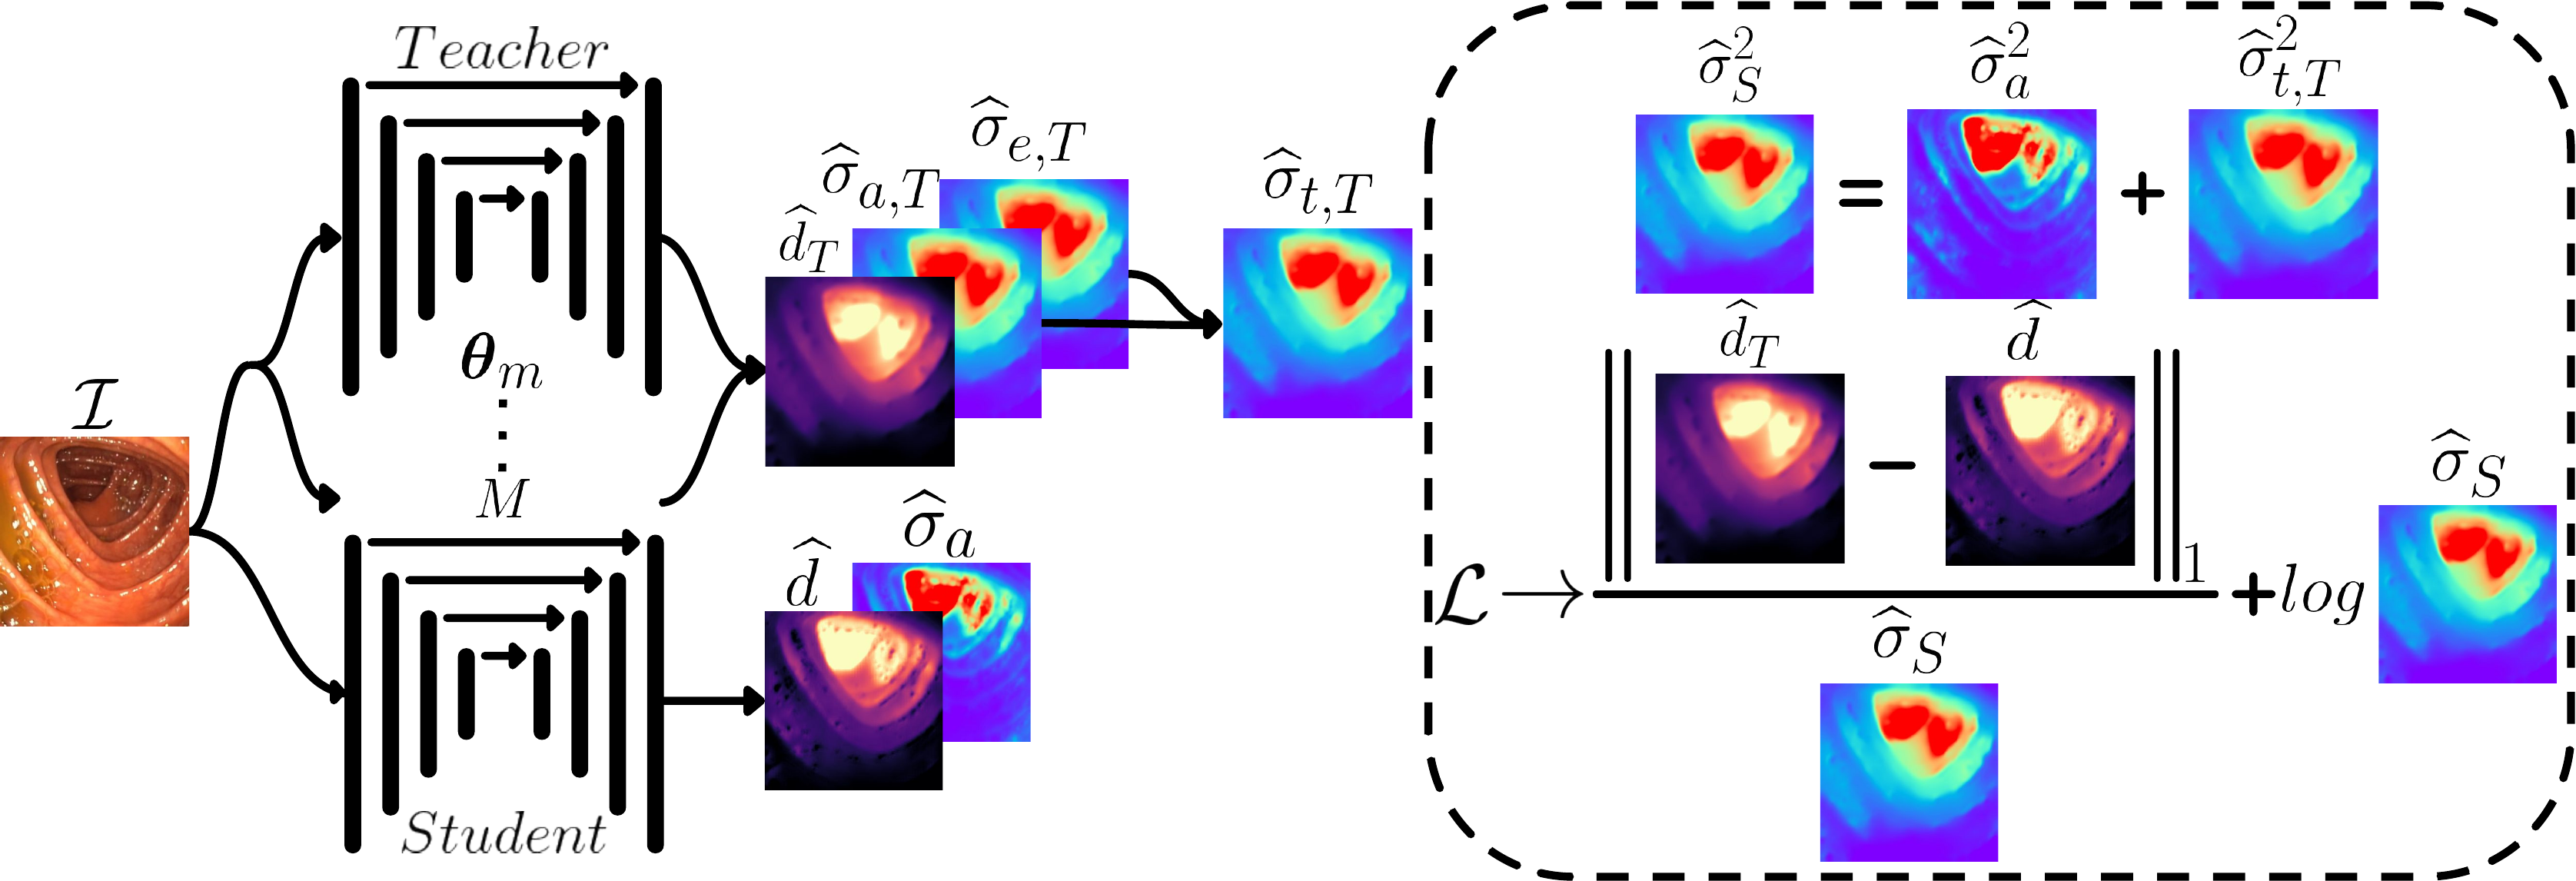}}
    
 \caption{Self-supervised training by a teacher-student approach. An ensemble of $M$ deep networks (teacher) supervises the training of a single encoder-decoder (student).
     Our contribution to improve the the state of the art is summing up the teacher's total uncertainty $\widehat{\sigma}_{t,T}$ to the aleatoric uncertainty issued by the student network $\widehat{\sigma}_{a}$ to obtain the depth error variance $\widehat{\sigma}_{S}$ that is included in the loss.
     }
    \label{fig:Approach_Teacher}
\end{figure}

\begin{figure}{\columnwidth}
  \centering
  \includegraphics[width=0.7\columnwidth]{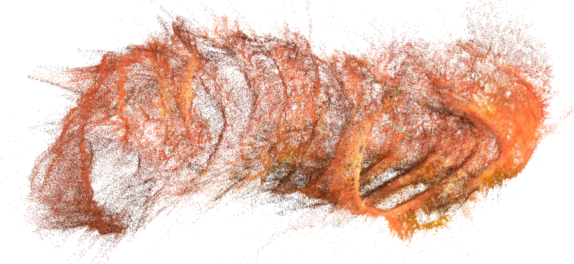}
  \caption{Multi-view reconstruction from the real colonoscopy images of the EndoMapper project using COLMAP.}
\end{figure}
\begin{figure}{\columnwidth}
  \centering
  \includegraphics[width=0.45\columnwidth,angle=90]{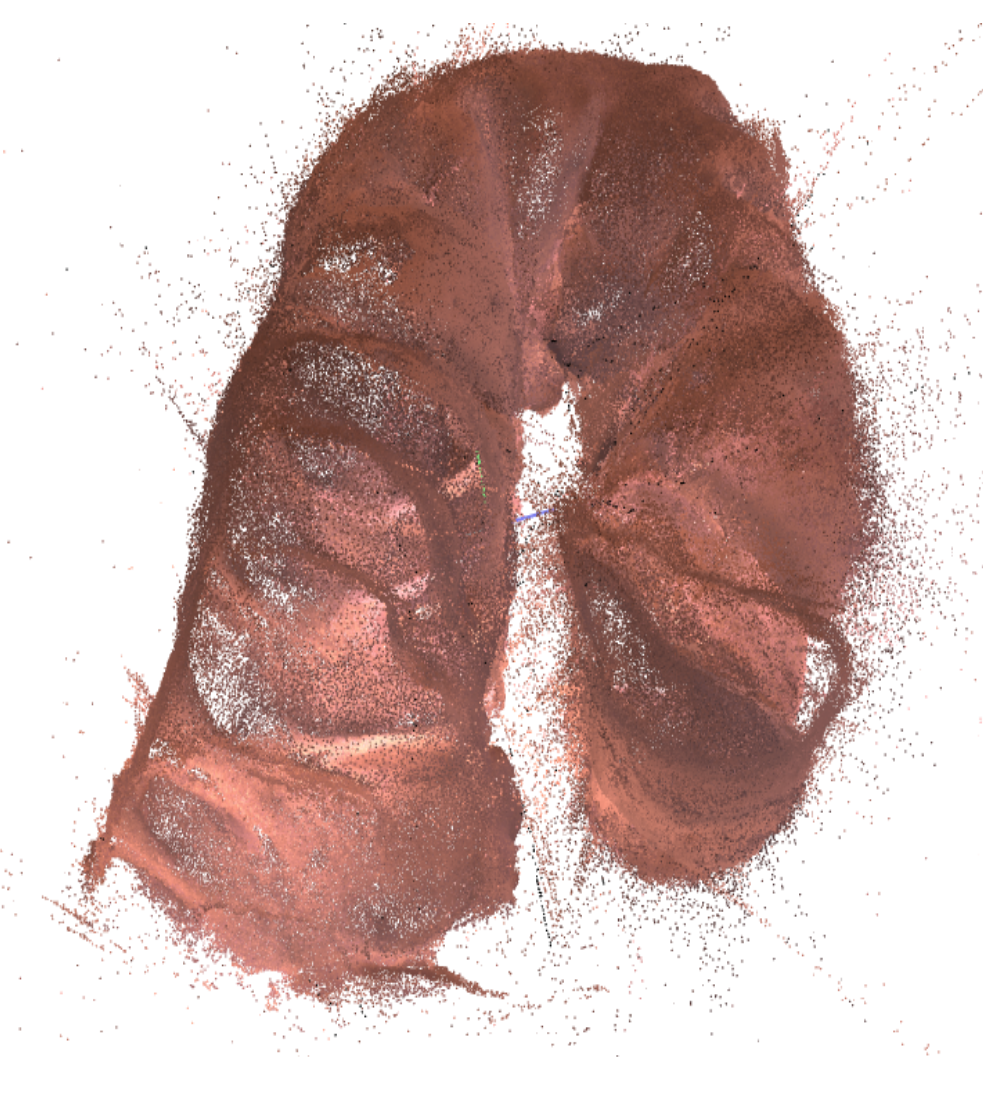}
  \caption{ Multi-view reconstruction from the colonoscopy synthetic images using COLMAP.
  }
    \label{fig:colmap-synth}
\end{figure}
